# Supplementary material for: Fierce selection and interference in B-cell repertoire response to chronic HIV-1
Source: arXiv:1802.08841 source file (2020-07-25)
Supplement: Supplementary file 1 [file SI.pdf]

# Supplementary Information

## 1 B-cell repertoire data

**HIV patients.** We analyze B-cell repertoire data from 6 HIV patients from ref. [1] with raw sequence reads accessible from the European Nucleotide Archive under study accession numbers, ERP009671 and ERP000572. We study the repertoire data in two untreated HIV patients with sample accession numbers, ERS664994 - 5001 (patient 1) and ERS139291- 9298 (patient 2) and in four patients with ART interruption at week 48, ERS664966 - 4974 (patient 3), ERS664975 - 4983 (patient 4), ERS664984 - 4992 (patient 5), ERS664976 - 5002 (patient 6). The data covers $\sim 2.5$ years of study with 6-8 sampled time points per patient; see Table S1 for details.

The B-cell repertoire sequences consist of 150bp non-overlapping paired-end reads (Illumina MiSeq), with one read covering much of the V gene and the other read covering the area around the CDR3 region and the J gene. For the initial processing of the raw reads we use pRESTO [2] (version 0.5.2) with the following steps: We filter sequences for quality ($> 32$) and length ($> 100$). The paired end reads that overlap are assumed to be anomalous, and are discarded from the analysis. We assemble the paired reads by aligning against the IMGT reference database of V genes [3], such that an appropriate size gap is inserted between the non-overlapping paired reads. Duplicate sequences are collapsed into unique sequences. The sequences contained a large number of singletons, that is sequences with no duplicates. With an R script, we calculate the minimum hamming distance of each singleton to any non-singleton, $H_0$. The distribution of $H_0$ is bimodal, and singletons with $H_0 < 5$ (the minimum between the modes) are discarded, since sequences with few changes are more likely to have appeared due to sequencing errors. Due to lack of barcoding for individual molecules, we only use the unique BCR sequences for analysis and do not incorporate the information on the multiplicity of each sequence.

**Healthy individuals.** We analyze memory B-cell repertoire data of 3 individuals published in ref. [4]: https://clients.adaptivebiotech.com/pub/robins-bcell-2016. The published data in healthy individuals is already preprocessed for quality control and corrected for sequencing error.

**BCR annotation.** In both datasets, we annotate the BCR repertoire sequences of each individual (pooled time points) by Partis [5]. Partis uses very large amounts of memory, so the initial (cache-parameters) stage is run on a subset of 200,000 random sequences, and the annotation stage is run on the full set of sequences. We process the output of Partis in R, which includes the estimated V gene/allele, J gene/allele, location of the CDR3 region, and an inferred naive sequence (germline before hyper-mutation). Sequences which have indels outside of the CDR3 are discarded. We partition the sequences into two groups: productive BCRs, which are in-frame and have no stop codons, and the unproductive BCRs. The sequences are further annotated by processing the inferred naive sequences with MiXCR [6, 7], which gives the CDR1, CDR2 and framework regions.

**Lineage reconstruction.** To identify BCR lineages, we first group sequences by the assigned V gene, J gene and CDR3 length, and then used single linkage clustering with a threshold of 90% hamming distance. A similar threshold has been previously suggested by ref. [8] to identify BCR lineages. Clusters of small size ($< 20$) are discarded from our analysis. For each cluster, there may be multiple inferred naive sequences, as this is an uncertain estimate, and the most common naive sequence is chosen to be the outgroup for genealogy reconstruction. See Table S1 for detailed statistics of BCR lineages in each individual.

**Unproductive BCRs.** Due to a larger sequencing depth in healthy individuals, we are able to reconstruct relatively large unproductive BCR lineages. Unproductive sequences are BCRs that were generated but due to a frameshift or insertion of stop codons were never expressed. These BCRs reside with productive (functional) BCRs in a nucleus and undergo hypermutation during B-cell replication, and therefore, provide a suitable null expectation for somatic

evolution during affinity maturation.

## 2 Inference of lineage phylogenies

**Lineage genealogy reconstruction.** For each lineage and its aligned sequences we reconstruct its underlying genealogical tree. We use FastTree [9] to construct the initial tree by maximum parsimony. We use this tree as seed for the maximum likelihood construction of the phylogeny with RAxML [10], using the GTRCAT substitution model. In the last step of tree topology reconstruction, we use the GTRGAMMA substitution model to optimize sequence divergence along the tree (i.e., branch lengths). We use a maximum likelihood approach to reconstruct nucleotide sequences of internal nodes on the tree [11]. We do not include the positions with gaps in the multi-sequence alignment in inference of tree topology and the nucleotide mutations along the tree.

We use the inferred naive sequence (germline) as the outgroup of the genealogy. The root of the tree may be some mutations away from the last common ancestor of the sampled sequences. This may be due to a number of initial rounds of hypermutation prior to secretion of the first selected B-cell, or alternatively, due to incorrect assignment of the germline allele during annotation; a fraction of V, D and J alleles circulating in the human population are missing from the existing reference datasets like IMGT [3]. In order to minimize the effect of such allele mis-assignments, we discard the mutations that separate the inferred germline sequence and the last common ancestor (root) of the tree from our analysis (i.e., mutations common to all sequences).

**Inference of branching time along a phylogeny.** To characterize the branch length statistics of lineages in units of divergence time (used in Fig. 2B and Fig. S1B), we use a maximum-likelihood approach and a probabilistic model to annotate internal nodes of a tree with times of occurrence, given the topology of the tree and the mutations on the branches. Internal nodes represent replication events, which may carry new mutations assigned to branches by the ancestral sequence reconstruction procedure. The model can also correct observation times of external nodes on the tree, given sufficient evidence. The model assumes a tree with $n$ nodes, $[o_1, \ldots, o_m, i_{m+1}, i_n]$, where $o_k$ are the sampled sequences in the leafs of the tree, and $i_k$ are the internal nodes of the tree. The observed nodes are annotated with their sampling times, $\mathbf{T} = [T_1, \ldots, T_m]$. Branches of the tree are annotated with their mutational distances, $\mathbf{d} = [d_1, \ldots, d_n]$. We only consider synonymous mutations for computation of mutational distances. The model estimates mutation rate, $\mu$ and the times $\mathbf{t} = [t_1, \ldots, t_n]$ of the nodes, by maximizing the likelihood:

$$P(\mathbf{d}, \mathbf{T}|\mathbf{t}, \mu) = \prod_{k=1}^{m} \frac{1}{\sigma\sqrt{2\pi}} \exp\left[-\frac{(t_k - T_k)^2}{2\epsilon}\right] \prod_{j=m+1}^{n} \frac{(\mu\tau_j)^d_j}{d_j!} \exp[\mu\tau_j], \quad (1)$$

where $\tau_j = t_j - t_{\mathcal{A}(j)}$, the time difference between a node in the tree and its parent, is constrained to be positive. The model assumes Gaussian measurement error with standard deviation $\sigma$ of the sampling time for the observed nodes, and the Poisson model for mutations on tree branches, with rate $\mu$. To limit the search space of the optimization algorithm we constrain the times $\mathbf{t}$ to be discrete; the units of time used in our data are weeks. Here we set $\sigma = 5$. The optimization is solved by an iterative procedure in which times of nodes are changed by one unit in the direction of score increase, until convergence.

## 3 Inference of selection from lineage tree statistics

We compare genealogies of B-cell lineages in HIV patients with healthy individuals to characterize the evolutionary selection during affinity maturation in response to chronic infection. Structure of genealogies has been linked to evolutionary modes in a population [12]. Rapid evolution under positive selection leads to skewed tree topologies

and elongated terminal branches [11, 13–15], compared to neutral evolution [12, 16] (Fig. S1A).

**Asymmetric tree branching.** We characterize the asymmetry of trees by the branching imbalance of the last common ancestor at the root of the tree - the last common ancestor may be a number of mutations away from the germline progenitor. We define the weight of each node in a tree by the number of leaves (terminal nodes) within its clade; see Fig. S1A [15]. The weight of the last common ancestor $w_{\text{anc.}}$, i.e., the total number of leaves in a tree, and its daughters, $w_{D_1}$, $w_{D_2}$, are indicated in the simulated trees of Fig. S1A. In rapid evolution under selection, the first branching event produces highly imbalanced sub-clades, and hence, extreme values for the weight of the first daughter nodes [15]. In contrast, neutral evolution predicts a uniform distribution of tree weights of ancestral sub-clades. Fig. 2A shows a U-shaped distribution of relative weights of daughters to the ancestor $w_D/w_{\text{anc.}}$ in lineages reconstructed from BCRs in HIV patients and in healthy individuals, indicating intra-lineage selection during affinity maturation.

**Terminal branch statistics.** In lineages under selection, the descendent sequences (leaves of a tree) are likely to coalesce to an ancestor with high fitness, resulting in long terminal branches in a tree (Fig. S1A) [14, 15] — branch length statistics are estimated in units of divergence time, rather than sequence hamming distance; see Section 2 of SI for inference of branching times along a phylogeny. In Fig. 2B we compare the ratio of mean terminal branch length of a lineage to the averaged length of all the branches in a lineage. The distribution of this branch length ratio in HIV patients show an excess of lineages with relatively long terminal branches, compared to the expected distribution for simulated neutral lineages of the same size (Kingman's coalescence); see Section 5 of SI. A similar trend with a weaker signal is seen in healthy individuals (Fig. 2B). To make sure that the strong signal in HIV patients is not only due to sampling of the repertoire over multiple time points, we repeat the same analysis on the subset of lineages which are sampled in only one time point. Fig. S1B shows a comparable over-representation of long terminal branches in this subset.

**Site frequency spectrum (SFS).** The SFS is the probability density $f(\nu)$ of observing a derived mutation (allele) with a given frequency $\nu$ in a lineage. A mutation that occurs along the phylogeny of a lineage forms a clade and is present in all the descendent nodes (leaves) of its clade (see Fig. S1A). Therefore, SFS carries information about the shape of the phylogeny, including both the topology and the branch lengths. In neutrality, mutations rarely reach high frequency, and hence, the SFS decays monotonically with allele frequency as, $f(\nu) \sim \nu^{-1}$ [16]. In phylogenies with skewed branching, many mutations reside on the larger sub-clade following a branching event, and hence, are present in the majority of the descendent leaves on the tree. The SFS of such lineages is often non-monotonic with an upturn in the high frequency part of the spectrum and a steeper drop ($\sim \nu^{-\beta}$ with $\beta > 1$) in the low frequency part of the spectrum [14]. To identify the targets of selection, we classify mutations based on the region they occur in. BCRs are made up of the three immunologically important complementarity-determining regions (CDRs) [17], CDR1, CDR2 and CDR3 and the remaining part of the V and J genes referred to as the framework region (FWR).

Fig. 2C shows SFS in lineages of HIV patients and in healthy individuals. We see a signifiant upturn of SFS polarized on non-synonymous mutations in pathogen-engaging CDR3 regions; this signal of selection is strongest in HIV patients with an order of magnitude increase in the high end of the spectrum (Fig. 2C). SFS polarized on mutations in other regions show steeper drop in the low frequency side of the spectrum compared to neutral expectation. Fig. S2 shows SFS of the unproductive BCR lineages in healthy individuals, with a comparable steep drop in low frequencies. A similar pattern of SFS has recently been reported for lineages of B-cell repertoires following influenza vaccination [18].

For analysis of lineage tree statistics, i.e., the weight imbalance, terminal branch statistics and SFS, we only rely on the relatively large lineages with size ($> 50$) leaves.

# 4 Selection and clonal interference likelihood ratios

**Selection likelihood ratio.** Hypermutations during affinity maturation create new clades within a lineage. The frequency $x$ of these clades change over time, as shown by the schematic in Fig. 3A. A mutation under positive (or negative) selection should reach a higher (lower) frequency than a neutral mutation. Many population genetics tests, such as the McDonnell-Kreitman test for positive selection [19], rely on a comparison between statistics of substitutions (i.e., mutations that fix within a population) and the circulating polymorphisms within species. Unlike phylogenies based on the species divergence, B-cell lineages form genealogies with many mutations that rise to intermediate frequencies as polymorphisms but often do not fix within a lineage. Here, instead of relying on the substitution statistics, we use the history of polymorphisms to quantify selection in B-cell lineages. In particular, we estimate the frequency propagator $G(x)$ [20] as the likelihood that a new mutation (allele) appearing in a lineage reaches frequency $x$ at some later time within a lineage (see schematic in Fig. 3A).

To estimate intra-lineage selection, we compare the likelihood of an amino acid changing non-synonymous mutation reaching a given frequency $x$ at any point in its time trace, $G(x)$ to that likelihood for a synonymous mutation in the same lineage, $G_0(x)$, and detemine the selection likelihood ratio (Fig. 3A) [20],

$$g(x) = \frac{G(x)}{G_0(x)}. \tag{2}$$

Due to heterogeneity and context dependence of mutation rates in different regions of BCRs, we evaluate the likelihood ratio separately for each region, namely the CDR3, CDR1 & CDR2 (pooled together) and framework regions (FWR). In the Fig. S5 we show the robustness of the region-specific selection likelihood ratio with respect to such mutational biases.

**Interference likelihood ratio (time-ordered selection).** Clonal competition among beneficial mutations on different genetic backgrounds is a characteristic of evolution in asexual populations. In the absence of clonal interference, beneficial mutations can readily fix in a population after they rise to intermediate frequencies, beyond which stochastic effects would not impact their fate [21]. Clonal interference reduces the efficacy of selection, resulting in a quasi-neutral regime of evolution [22].

To examine the amount of clonal competition among BCRs of a lineage, we consider time ordered selection propagators (interference propagators) indicating the likelihood that a mutation reaches frequency $x$ and later goes extinct, $H(x) = G(x) \times G(0|x)$; here $G(0|x)$ is the conditional probability that a mutation trajectory decays to frequency 0 given that it starts from frequency $x$; see schematic in Fig. 3A. We estimate the interference likelihood ratio by comparing the probability of a non-synonymous mutation to reach a frequency $x$ and later go extinct $H(x)$ to the same scenario for synonymous mutations, $H_0(x)$ (Fig. 3A),

$$h(x) = \frac{H(x)}{H_0(x)} \equiv \frac{G(x) \times G(0|x)}{G_0(x) \times G_0(0|x)}. \tag{3}$$

**Fraction of selected mutations based on the likelihood ratios.** Following the well established tradition of population genetics, we assume that synonymous mutations that do not change the amino acid provide a neutral gauge for evolution. In the case of frequency $x = 1$ the propagator ratio $g(x)$ becomes equal to the ratio of the fixation probability $(d/n)\Big/(d_0/n_0)$ where $d$ and $d_0$ are respectively the number of fixed non-synonymous and synonymous polymorphisms and $n$ and $n_0$ are total number of polymorphisms is each class. In other words, $g(x = 1)$ is equivalent to the McDonald-Kreitman test for selection based on the observed polymorphisms [19].

Selection likelihood ratio $g(x) = G(x)/G_0(x)$ larger than 1 implies an over-representation of non-synonymous compared to synonymous changes that reach frequency $x$ and is indicative of beneficial amino acid changes in a

given region. Assuming a total of $N$ non-synonymous mutations, we expect $NG_0(x)$ of these mutations to reach frequency $x$ by neutral evolution, and at least a fraction $\alpha_{\text{benef.}}(x) = (N(x) - NG_0(x))/N(x) = (g(x) - 1)/g(x)$ of these mutations to be beneficial [23]. On the other hand, a selection likelihood ratio smaller than 1 indicates negatively selected amino acid changes in a given region. The deviation from the expected number of non-synonymous mutations in neutrality, $NG_0(x) - N(x)$, is an estimate for the number of mutations that were suppressed due deleterious fitness effects, indicating that at least a fraction $\alpha_{\text{del.}}(x) = 1 - g(x)$ of non-synonymous mutations to be under negative selection [23]. Similarly, we can compute the fraction of beneficial and deleterious mutations that are impacted by clonal interference, $\kappa_{\text{benef.}}(x) = (h(x) - 1)/h(x)$ for $h(x) > 1$, and $\kappa_{\text{del.}}(x) = 1 - h(x)$ for $h(x) < 1$.

**Robustness of selection inference.** It should be noted that the heterogenous and context dependent somatic hyper-mutation rates during affinity maturation [24–28] introduce BCR-specific biases that could influence inference of selection. In order to verify the robustness of our method, we have simulated the process of affinity maturation based on two distinct BCR-specific hyper-mutation models [24,26,28] along the inferred BCR lineage phylogenies; see Section 5 of SI for details. Fig. S5 shows that the region-specific likelihood ratios $g(x)$, $h(x)$ are insensitive to the heterogenous hyper-mutation statistics and such biases do not produce spurious evidence for selection and clonal interference. In addition, the likelihood ratio is insensitive to the initial frequency of an allele within a lineage [20] and provides a robust measure for inference of selection in evolving genealogies.

**Inference of likelihood ratio statistics from data.** The descendants of a given mutation $\alpha$ on a lineage tree define the clade $\mathcal{C}^\alpha$. We evaluate the frequency of mutation $\alpha$ at time $t$, $x^\alpha(t)$ as the fraction of the observed sequences (leaves of the tree) from time point $t$ that reside within the clade $\mathcal{C}^\alpha$. The fraction of non-synonymous and synonymous mutations that reach frequency $x$ during their history define the selection propagators $G(x)$ and $G_0(x)$, respectively. To infer statistically significant evidence for selection, we estimate propagators based on the mutations pooled from lineages of common gene classes, e.g. lineages with common V gene (Fig. 3B) or common V & J genes (Fig. 3C and Fig. S4). We evaluate the expected error of a propagator at frequency $x$, by assuming binomial sampling from the total of $N$ non-synonymous and $N_0$ synonymous mutations (i.e., all the mutations observed in a given gene class). This results in the sampling errors $\sigma^2(x) = G(x)(1 - G(x))/N$ for non-synonymous and $\sigma_0^2(x) = G_0(x)(1 - G_0(x))/N_0$ for synonymous mutations, and a corresponding propagated error for the ratio, $g(x)$ in eq. 2. We use a similar approach to estimate the error for the interference likelihood ratio, $h(x)$ in eq. 3.

# 5 Simulations

**Simulated trees.** In Fig. 2B, we compare the branch length characteristics of the BCR genealogies with the neutral expectation from 2000 simulated trees with Kingman's coalescence, generated by the beta coalescent algorithm with parameter $\alpha = 1$ [29]. The sizes of the simulated trees in the neutral ensemble are drawn from the BCR lineage size distribution in HIV patients. The schematic trees in Fig. S1A are also generated similarly by the beta coalescent algorithm [29] with parameters $\alpha = 1$ for neutral evolution and $\alpha = 2$ for rapid adaptation.

**Null model for context-dependent affinity maturation.** We simulate mutations along BCR lineage trees according to two context-dependent models of hyper-mutation, (i) IGoR statistics [28] and (ii) S5F [24]. For a given branch on a lineage tree, we draw a number of mutations equal to the branch length from a multinomial distribution with position-specific weights determined by the hypermutation models. Due to the changes in the sequence, we update the position weights at each internal node of the tree to account for context-dependent hyper-mutation rates. This procedure reshuffles the identify of mutations along BCRs according to the neutral hyper-mutation models, while preserving the shape of tree. Fig. S5 shows that the propagator statistics do not recover evidence for region-specific selection in BCRs in the simulated lineages. Therefore, the original selection signal in Fig. 3 is not

reflecting any spurious effect due to heterogenous mutation rates.

## Supplemental references


[1] Hoehn KB, Gall A, Bashford-Rogers R, Fidler SJ, Kaye S, et al. (2015) Dynamics of immunoglobulin sequence diversity in HIV-1 infected individuals. Phil Trans R Soc B 370.

[2] Vander Heiden JA, Yaari G, Uduman M, Stern JNH, O'Connor KC, et al. (2014) pRESTO: a toolkit for processing high-throughput sequencing raw reads of lymphocyte receptor repertoires. Bioinformatics 30: 1930–1932.

[3] Lefranc MP, Lefranc G (2001) The Immunoglobulin FactsBook. Academic Press.

[4] DeWitt WS, Lindau P, Snyder TM, Sherwood AM, Vignali M, et al. (2016) A Public Database of Memory and Naive B-Cell Receptor Sequences. PLoS ONE 11: e0160853.

[5] Ralph DK, Matsen FA (2016) Consistency of VDJ Rearrangement and Substitution Parameters Enables Accurate B Cell Receptor Sequence Annotation. PLoS Comput Biol 12: e1004409.

[6] Bolotin DA, Poslavsky S, Mitrophanov I, Shugay M, Mamedov IZ, et al. (2015) MiXCR: software for comprehensive adaptive immunity profiling. Nat Methods 12: 380–381.

[7] Bolotin DA, Poslavsky S, Davydov AN, Frenkel FE, Fanchi L, et al. (2017) Antigen receptor repertoire profiling from RNA-seq data. Nat Biotechnol 35: 908–911.

[8] Gupta NT, Adams KD, Briggs AW, Timberlake SC, Vigneault F, et al. (2017) Hierarchical Clustering Can Identify B Cell Clones with High Confidence in Ig Repertoire Sequencing Data. J Immunol 198: 2489–2499.

[9] Price MN, Dehal PS, Arkin AP (2010) FastTree 2–approximately maximum-likelihood trees for large alignments. PLoS ONE 5: e9490.

[10] Stamatakis A (2014) RAxML version 8: a tool for phylogenetic analysis and post-analysis of large phylogenies. Bioinformatics 30: 1312–1313.

[11] Neher RA, Russell CA, Shraiman BI (2014) Predicting evolution from the shape of genealogical trees. eLife 3: e03568.

[12] Wakeley J (2007) Coalescent Theory: an introduction. Roberts Publishers.

[13] Desai MM, Walczak AM, Fisher DS (2013) Genetic diversity and the structure of genealogies in rapidly adapting populations. Genetics 193: 565–585.

[14] Neher RA, Hallatschek O (2013) Genealogies of rapidly adapting populations. Proc Natl Acad Sci USA 110: 437–442.

[15] Dayarian A, Shraiman BI (2014) How to infer relative fitness from a sample of genomic sequences. Genetics 197: 913–923.

[16] Kingman J, 1982 On the genealogy of large populations, in "Essays in Statistical Science"(J. Gani and EJ Hannan, Eds.) J 19: 27–43.

[17] Janeway CA, Travers P, Walport M, Shlomchik M (2005) Immunobiology: the immune system in health and disease (Garland Science, New York).

[18] Horns F, Vollmers C, Dekker CL, Quake SR (2017) Signatures of selection in the human antibody repertoire: selective sweeps, competing subclones, and neutral drift. bioRxiv doi.org/10.1101/145052.

[19] McDonald JH, Kreitman M (1991) Adaptive protein evolution at the Adh locus in Drosophila. Nature 351: 652–654.

[20] Strelkowa N, Lässig M (2012) Clonal interference in the evolution of influenza. Genetics 192: 671–682.

[21] Desai MM, Fisher DS (2007) Beneficial mutation–selection balance and the effect of linkage on positive selection. Genetics 17: 385–394.

[22] Schiffels S, Szöllősi GJ, Mustonen V, Lässig M (2011) Emergent neutrality in adaptive asexual evolution. Genetics 189: 1361–1375.

[23] Smith NGC, Eyre-Walker A (2002) Adaptive protein evolution in Drosophila. Nature 415: 1022–1024.

[24] Yaari G, Vander Heiden JA, Uduman M, Gadala-Maria D, Gupta N, et al. (2013) Models of somatic hypermutation targeting and substitution based on synonymous mutations from high-throughput immunoglobulin sequencing data. Front Immunol 4: 358.

[25] Yaari G, Benichou JIC, Vander Heiden JA, Kleinstein SH, Louzoun Y (2015) The mutation patterns in B-cell immunoglobulin receptors reflect the influence of selection acting at multiple time-scales. Philos Trans R Soc Lond, B, Biol Sci 370: 20140242.

[26] Elhanati Y, Sethna Z, Marcou Q, Callan CG, Mora T, et al. (2015) Inferring processes underlying B-cell repertoire diversity. Phil Trans R Soc B 370.

[27] Hoehn KB, Lunter G, Pybus OG (2017) A phylogenetic codon substitution model for antibody lineages. Genetics 206: 417–427.

[28] Marcou Q, Mora T, Walczak AM (2017) IGoR: a tool for high-throughput immune repertoire analysis .

[29] Neher RA, Kessinger TA, Shraiman BI (2013) Coalescence and genetic diversity in sexual populations under selection. Proc Natl Acad Sci USA 110: 15836–15841.

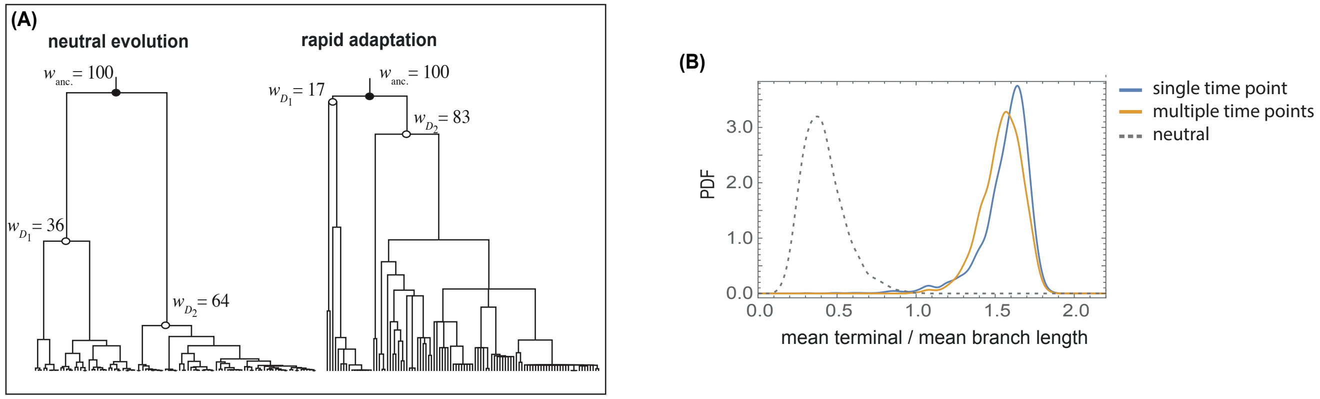


Figure S1: **Impact of selection on lineage tree statistics. (A)** Simulated phylogenies for neutral evolution (left) and rapid adaptation with positive selection (right), generated by the coalescence package [29] and plotted with FastTree [9]. The weights of the ancestral node $w_{\mathrm{anc.}}$ and its daughters $w_{D_1}$, $w_{D_2}$ (i.e., their clone size) are indicated in each phylogeny. **(B)** Branch length statistics for lineages sampled in only one time point from HIV patients. The distribution of mean terminal branch length (in units of divergence time) relative to the mean length of all branches is comparable between BCR lineages of HIV patients that are present in only a single time point (blue) and lineages sampled over multiple time points (orange). The corresponding distribution for the simulated neutral trees (similar to Fig. 2B) is shown by a dotted line. The elongated terminal branches in BCR lineages is indicative of positive selection.

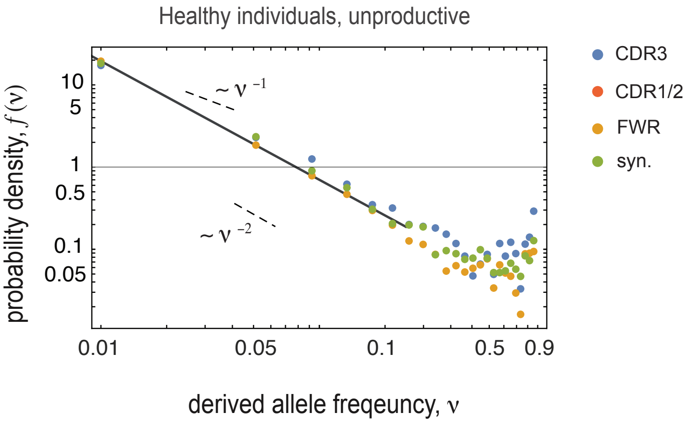


Figure S2: **Site frequency spectrum of the unproductive BCR lineages.** SFS $f(\nu)$ is shown for mutations in different regions of BCRs (distinct colors) in unproductive lineages of healthy individuals; see Fig. 2C for SFS of productive lineages.

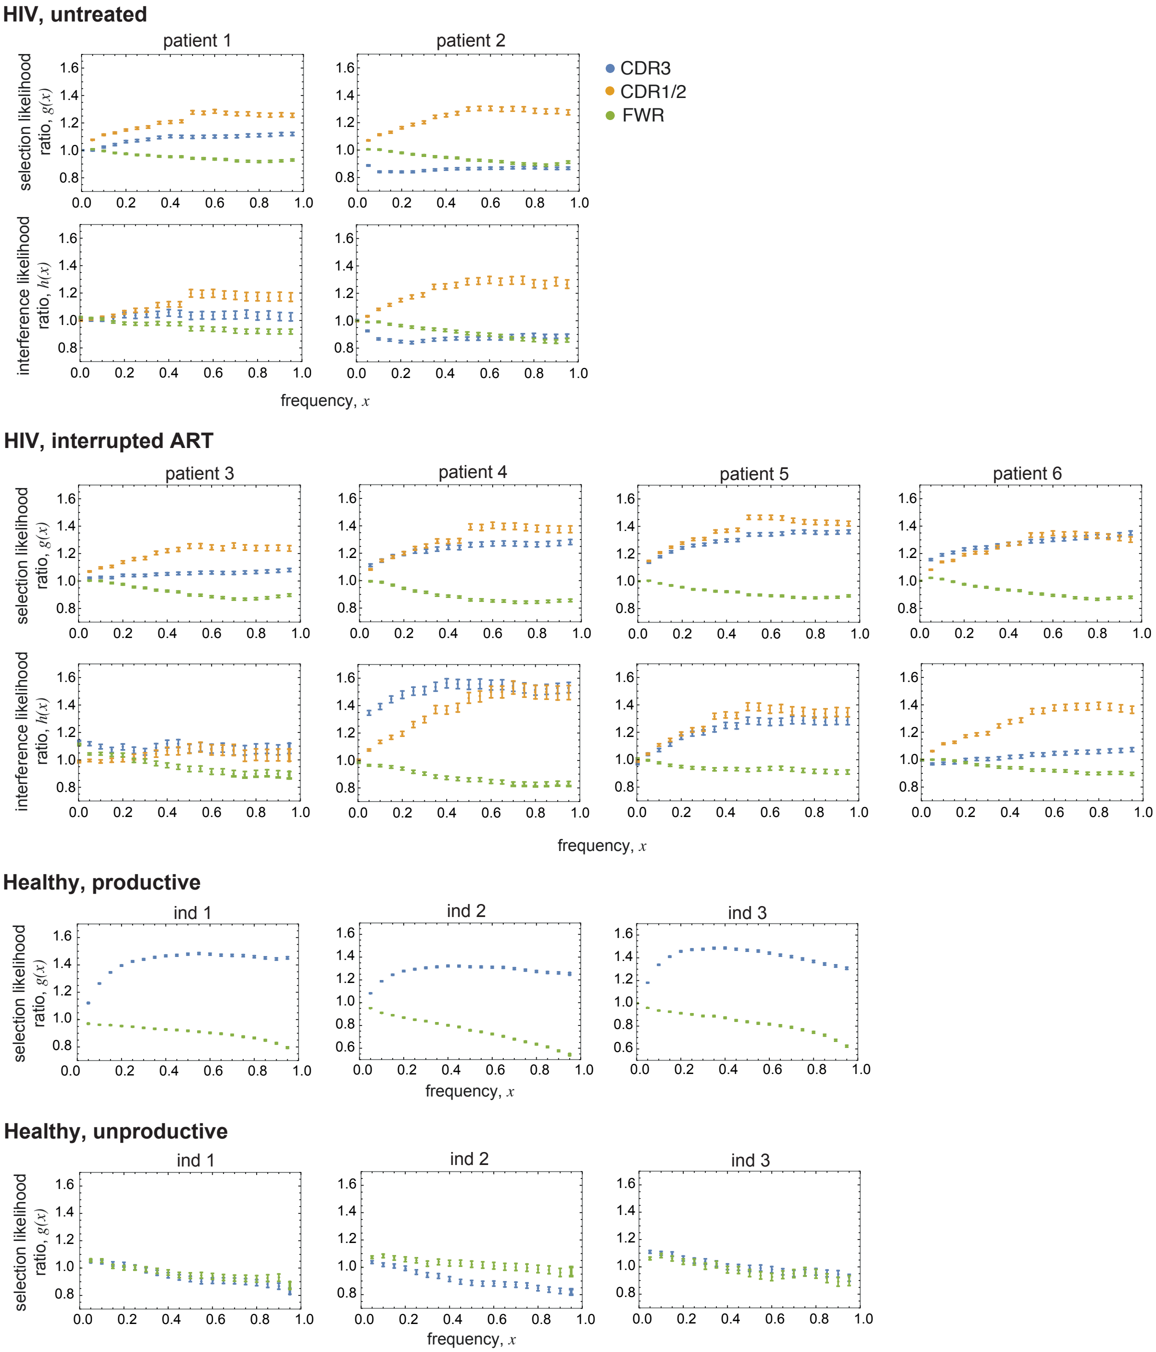


Figure S3: **Selection and interference likelihood ratios in all individulas.** Panels show selection and interference likelihood ratios $g(x)$, $h(x)$ in HIV patients (untreated and with interrupted ART) and the selection likelihood ratio $g(x)$ in productive and unproductive lineages of healthy individuals, estimated from all lineages in each individual. We consistently see strong evidence for negative selection in FWR regions of productive lineages and positive selection in both or either of CDR regions. We do not see such distinction in unproductive lineages. Note that the repertoire level averaged likelihood ratios are highly coarse grained statistics and miss the gene-specific evidence for selection and clonal interference, as shown in Fig. 3.

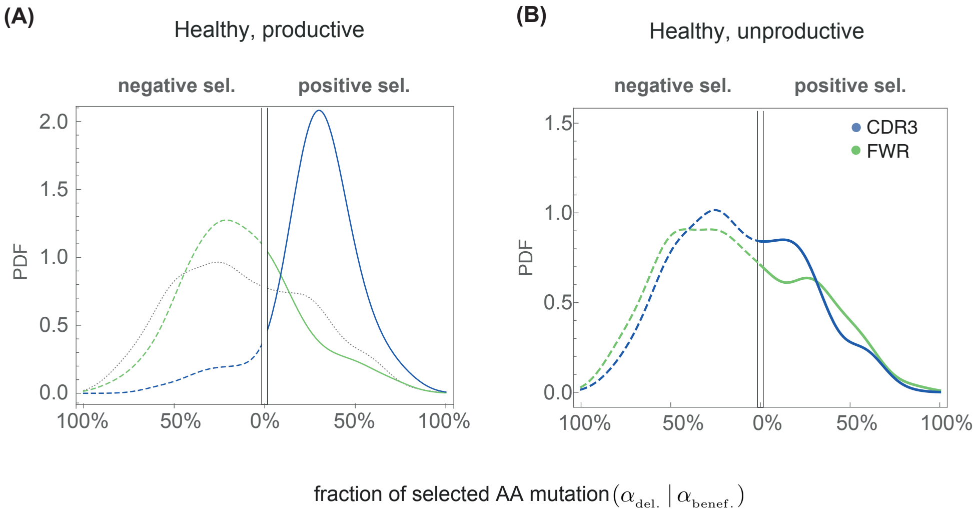


Figure S4: **Fraction of selected BCR mutations in healthy individuals.** The probability density across distinct VJ-gene classes for the (minimum) fraction of beneficial (right) $\alpha_{\mathrm{benef.}}$ and deleterious (left; inverted x-axis) $\alpha_{\mathrm{del.}}$ amino acid changes that reach frequency $x = 80\%$ within a lineage is shown for different regions of BCRs in **(A)** productive and **(B)** unproductive lineages of healthy individuals. Similar to HIV patients (Fig. 3), the CDR3 mutations in productive lineages of healthy individuals are under positive selection, whereas the FWR mutations are under negative selection. We do not infer any significant differences between selection patterns in CDR3 and in FWR region of unproductive lineages. The probability density for mutations pooled from both regions of unproductive lineages is shown as the null expectation (dotted gray line), similar to Fig. 3.

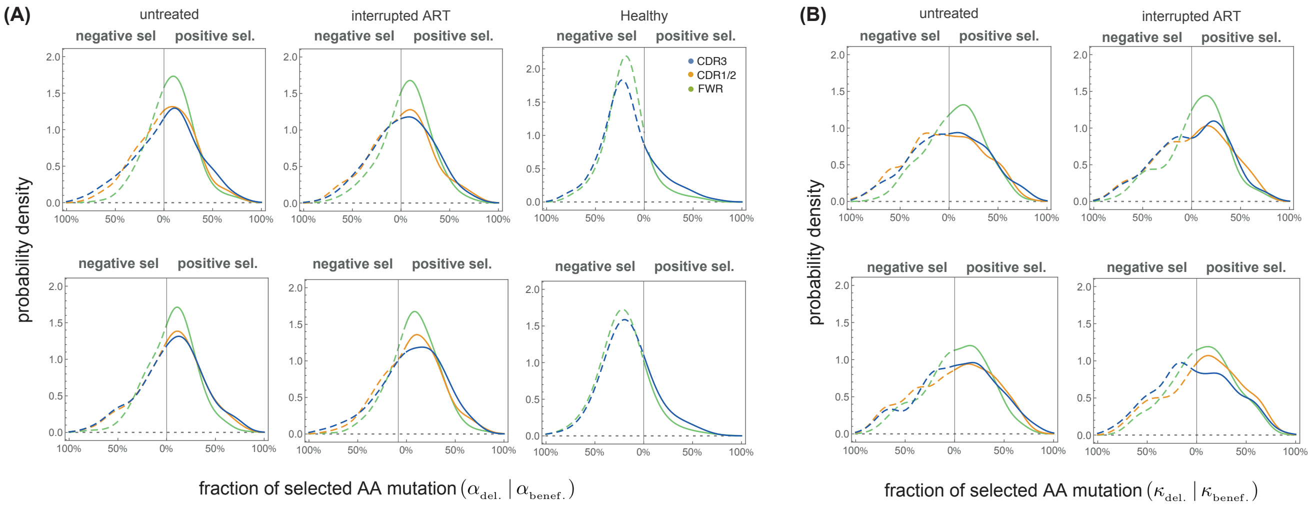


Figure S5: **Robustness of selection inference to BCR hypermutation biases.** The figure shows the statistics of selected mutations for simulated neutral hypermutation processes along the inferred B-cell lineages, as described in Section 5 of SI. We use two hypermutation models, IGoR statistics [28] (top row) and the S5F model [24] (bottom row). Similar to Fig. 3, each panel shows the probability density across distinct VJ-gene classes for **(A)** the minimum fraction of beneficial / deleterious mutations ($\alpha_{\mathrm{benef.}}$ / $\alpha_{\mathrm{del.}}$) that reach frequency $x = 80\%$, and (**B**) for beneficial / deleterious mutation fractions ($\kappa_{\mathrm{benef.}}$ / $\kappa_{\mathrm{del.}}$) that reach frequency $x = 60\%$ and later go extinct. These statistics are estimated for mutations in different regions of BCRs (colors) in healthy individuals, HIV patients with interrupted ART and in untreated HIV patients. The region-specific pattern of selection seen in Fig. 3 is simulated lineages with context-dependent hypermutation models.

| | | HIV infected (untreated ) | | HIV infected (interrupted ART at week 48) | | | | Healthy | | |
|---|---|---|---|---|---|---|---|---|---|---|
| | | patient 1 | patient 2 | patient 3 | patient 4 | patient 5 | patient 6 | ind 1 | ind 2 | ind 3 |
| | size | | | | | | | | | |
| # productive lineages | $> 20$ | 3,335 | 3,702 | 3,164 | 2,125 | 4,342 | 4,155 | 21,486 | 15,755 | 15,782 |
| | $> 50$ | 785 | 773 | 613 | 485 | 1,246 | 1,205 | 5,242 | 3,978 | 3,390 |
| # unproductive lineages | $> 20$ | 0 | 0 | 0 | 0 | 0 | 0 | 897 | 1041 | 962 |
| | $> 50$ | 0 | 0 | 0 | 0 | 0 | 0 | 177 | 198 | 155 |
| time samples (weeks) | | 0, 4, 16, 24, 52, 72, 120 | 0, 4, 12, 16, 24, 52 60, 108 | 4, 12, 16, 24, 52, 60, 108 | 4, 12, 16, 24, 52, 60, 108 | 4, 12, 16, 24, 52, 60, 108 | 0, 4, 16, 24, 52, 60, 108 | 0 | 0 | 0 |

Table S1: Statistics of reconstructed BCR lineages with size $(> 20)$ and $(> 50)$ and the sampled time points after the start of the study in HIV infected patients and in healthy individuals.
